# Supplementary material for: Modeling inclusive electron-nucleus scattering with Bayesian artificial neural networks
Source: arXiv:2406.06292 source file (2024-06-10)
Supplement: Supplementary file 1 [file supplement.pdf]

# Supplemental Material

Joanna E. Sobczyk, Noemi Rocco, Alessandro Lovato

[a]Institut für Kernphysik and PRISMA+ Cluster of Excellence, Johannes Gutenberg-Universität, 55128, Mainz, Germany,
[b]Theoretical Physics Department Fermi National Accelerator Laboratory P.O. Box 500 Batavia Illinois 60510 USA
[c]Physics Division Argonne National Laboratory Argonne IL 60439
[d]INFN-TIFPA Trento Institute of Fundamental Physics and Applications 38123 Trento Italy

## 1. Additional data on inclusive cross sections

In Figures 1 and 2 we show a comparison of the ANN against the entire test dataset. These 34 kinematic setups cover all the nuclei considered in this work, including $^6$Li, for which there are only three datasets available. These setups also span many orders of magnitude and comprise various physical reaction mechanisms, ranging from the elastic transition to the deep inelastic scattering region. It is worth pointing out that both $^6$Li and $^{16}$O cross-sections are predicted remarkably well, despite the ANN being trained only on two ($^6$Li) and four ($^{16}$O) kinematics. Hence, the ANN learns features from other nuclei and is able to provide reasonable predictions in regions where experimental data are scarce. As expected, this procedure leads to a somewhat larger uncertainty band. A similar pattern emerges for the low-energy datasets on $^{12}$C ($E$ = 0.16 GeV, $\theta$ = 36°) and ($E$ = 0.20 GeV, $\theta$ = 36°). Lastly, we also observe some low-lying peaks, particularly for $^4$He. This part of the spectrum, where transitions to excited states are important, is burdened with much larger error due to insufficient available data. This behavior is consistent with our results for the longitudinal and transverse responses.

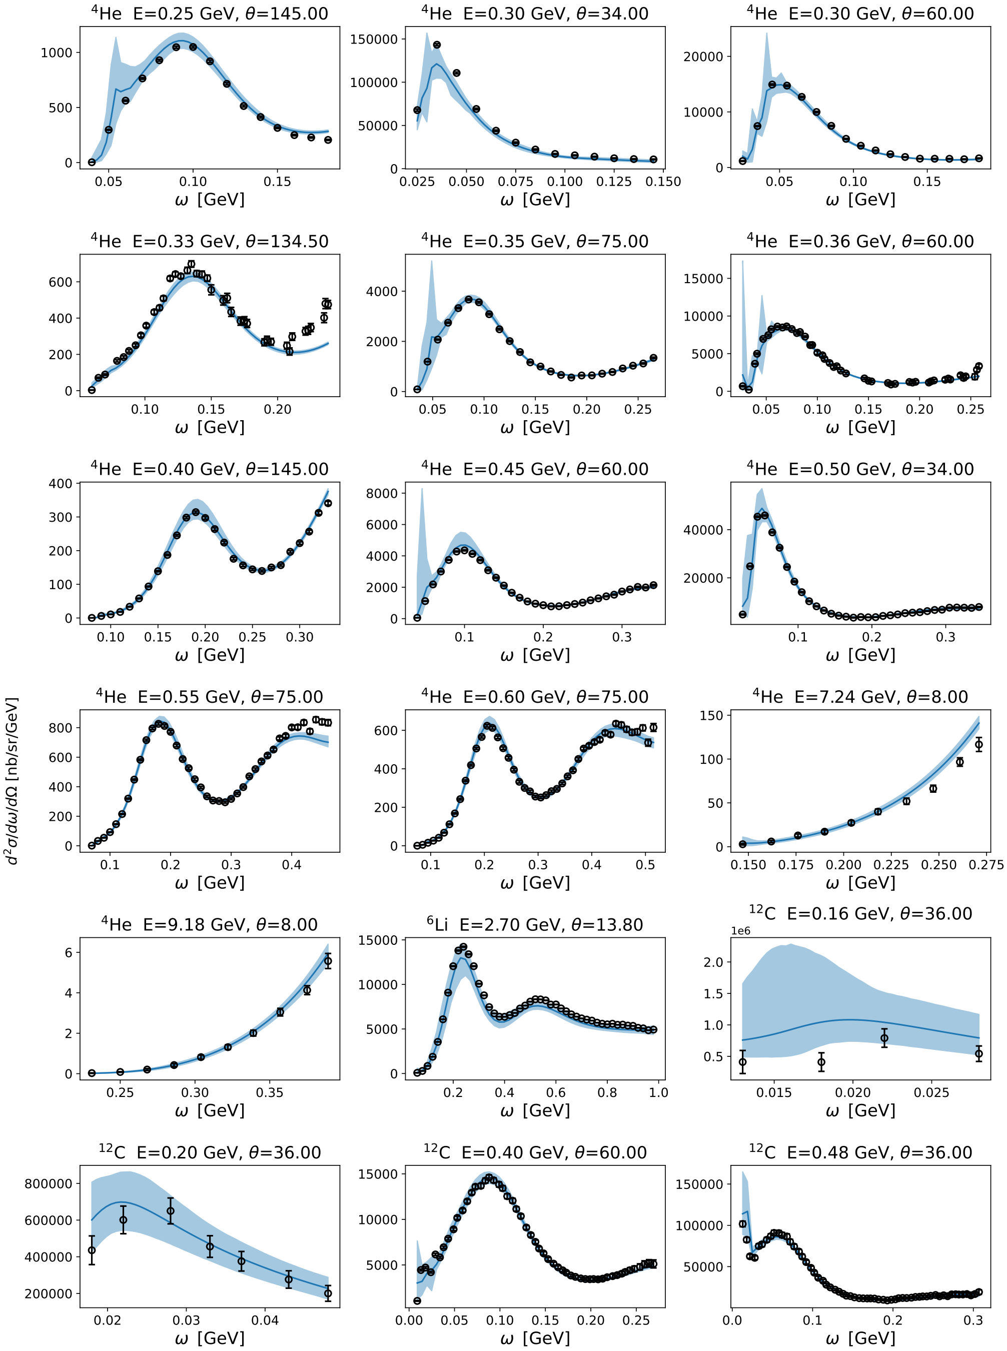


Figure 1: Prediction on the test datasets for $^4$He, $^6$Li and $^{12}$C.

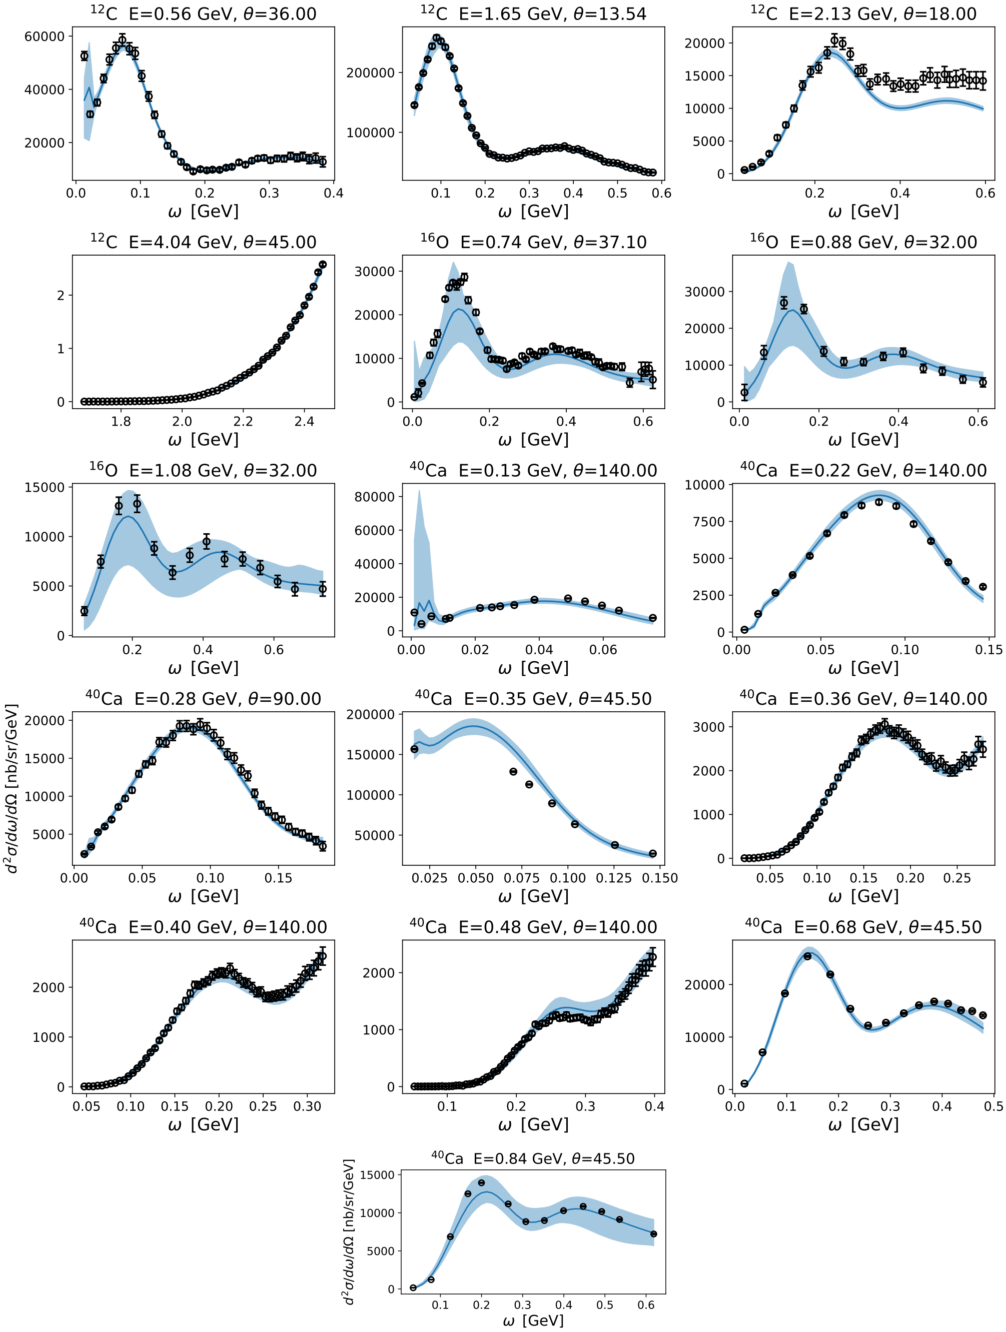


Figure 2: Prediction on the test datasets for $^{12}$C, $^{16}$O and $^{40}$Ca.

## 2. Additional comparisons with Rosenbluth-separation analyses

We provide additional predictions of the ANN for the electromagnetic responses of $^{4}$He, $^{12}$C, and $^{40}$Ca for the kinematics where Rosenbluth separation data are available in the literature.

The ANN responses of $^{4}$He, displayed in Figure 3, are in excellent agreement with the Rosenbluth separation analyses, and they share some distinctive features with the latter. The ANN extraction of the responses generally exhibits smaller uncertainties in the transverse channel than in the longitudinal, where the uncertainties tend to grow with the magnitude of the momentum transfer. At low energy transfers, the uncertainties in the predictions are large due to the elastic contribution and transitions to low-lying excited states, reducing the precision of the ANN responses. This behavior is primarily due to the scarcity of experimental data at low energies, which is insufficient to constrain the parameters of the ANN. Additionally, because the contributions from elastic and low-lying transitions strongly depend on the specific nuclear target, the ANN cannot leverage information from one nucleus to predict responses for a different one.

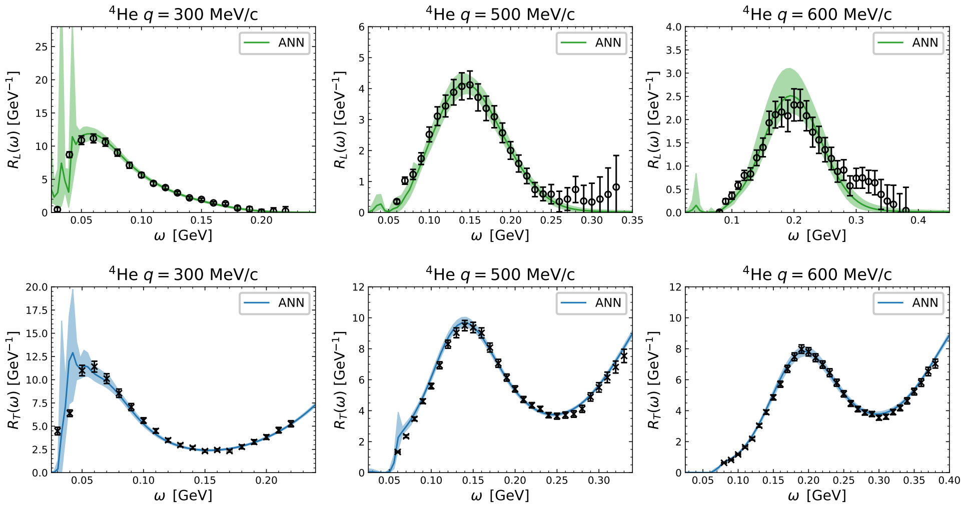


Figure 3: Rosenbluth separation for $^{4}$He at $q = 300,\ 500,\ 600$ MeV/c. Data taken from Carlson et al. (2002).

Similar trends are observed in $^{12}$C and $^{40}$Ca, shown in 4. We note however that the ANN transverse response of $^{40}$Ca consistently overestimates the Rosenbluth-separation data from Jourdan (1996). In the following, we investigate closer the source of this discrepancy.

*Rosenbluth separation for $^{40}$Ca*

Experimental electron scattering on $^{40}$Ca was primarily measured at two facilities: Saclay Meziani et al. (1984) and MIT-Bates Williamson et al. (1997), collecting 1016 and 296 data- points respectively. Both experiments performed the Rosenbluth separation at several values of momentum transfer, leading to different results. Later Jourdan (1996) re-examined the data taking all available measurements into account.

We employed our ANN to investigate the source of discrepancy between the two experiments and to assess how our predictions depend on the datasets used in the training. In Fig. 5, we show

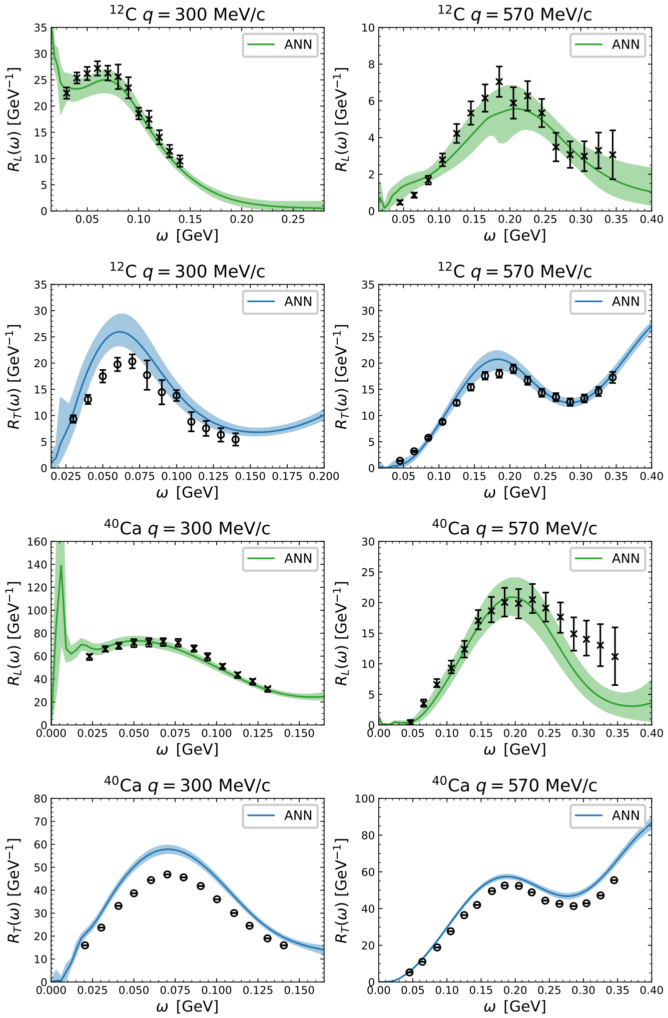


Figure 4: Rosenbluth separation for $^{12}$C and $^{40}$Ca at $q = 380,\ 570$ MeV/c. Data taken from Jourdan (1996).

our predictions where we restrict the training datasets to either Saclay or Bates data. As we can see, our results coincide with the Rosenbluth separation performed by each experiment.

When using the datasets combined, our ANN tends more towards Saclay predictions, since this experiment provides over three times more data points. In addition, we find a $q$-dependence in the discrepancy between both Rosenbluth-separation analyses. For instance, in Fig. 5, we show results for $q = 300$ MeV/c, where the discrepancy is considerably smaller for the longitudinal response.

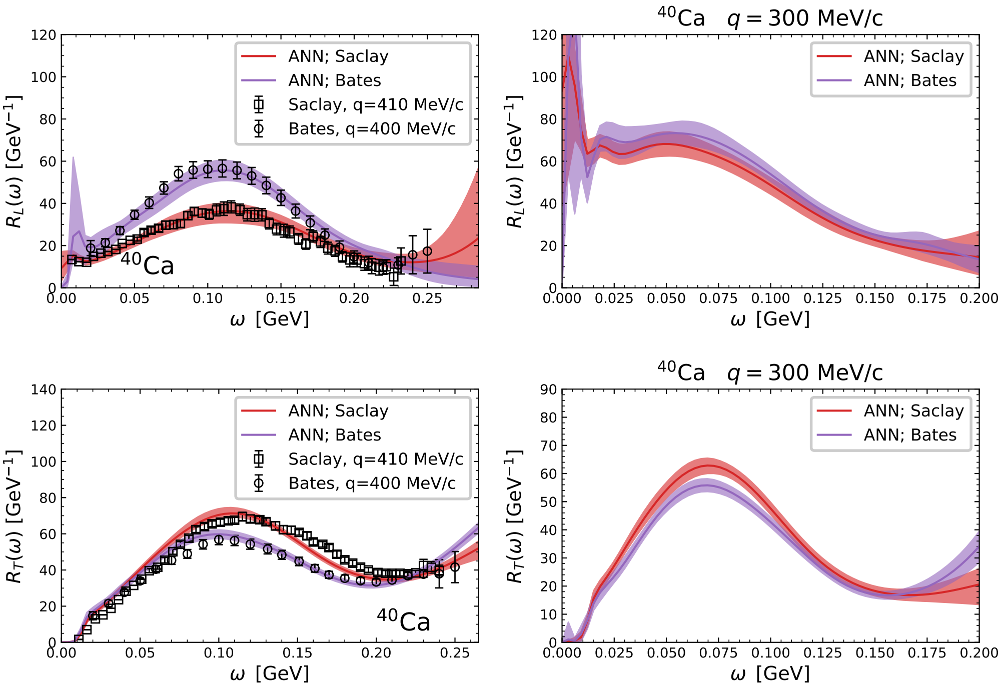


Figure 5: The ANN predictions when for $^{40}$Ca only data from a single experiment were used for training. Data taken from Meziani et al. (1984) and Williamson et al. (1997). In the left column we show our results compared to the Rosenbluth separation performed by each experiment for a similar momentum transfer $q$ = 400 MeV/c (Bates) and $q$ = 410 MeV/c (Saclay). In the right column we compare both predictions at $q$ = 300 MeV/c.

## References


Carlson, J., Jourdan, J., Schiavilla, R., Sick, I., 2002. Longitudinal and transverse quasielastic response functions of light nuclei. Phys. Rev. C 65, 024002. doi:10.1103/PhysRevC.65.024002, arXiv:nucl-th/0106047.

Jourdan, J., 1996. Quasielastic response functions: The Coulomb sum revisited. Nucl. Phys. A 603, 117–160. doi:10.1016/0375-9474(96)00143-1.

Meziani, Z.E., et al., 1984. Coulomb Sum Rule for Ca-40, Ca-48, and Fe-56 for |q (Vector)| <= 550-MeV/c. Phys. Rev. Lett. 52, 2130–2133. doi:10.1103/PhysRevLett.52.2130.

Williamson, C.F., et al., 1997. Quasielastic electron scattering from Ca-40. Phys. Rev. C 56, 3152–3172. doi:10.1103/PhysRevC.56.3152.
